# Supplementary material for: lassopack: Model selection and prediction with regularized regression in Stata
Source: arXiv:1901.05397 source file (2019-01-16)
Supplement: Supplementary file 1 [file main_appendix.tex]

Appendix goes here.
\section{Tables}
\begin{table}[H]
\centering
    \begin{tabular}{lll}
    \hline\hline
                        
     & \multicolumn{2}{c}{Definition of $X$-independent $\lambda_0$}
     \\
     & lasso & square-root lasso   \\
    \hline
     $X$-independent
     & \multirow{2}{*}{$2c\sqrt{n}\Phi^{-1}(1-\gamma/(\log(n)2p))$}
     & \multirow{2}{*}{$c\sqrt{n}\Phi^{-1}(1-\gamma/(\log(n)2p))$}
     \\
     \emph{(default)}&&\\
     $X$-independent 
     & \multirow{2}{*}{$2c\sqrt{n}\sqrt(2\log(2p/(\gamma/\log(n)))$}
     & \multirow{2}{*}{$c\sqrt{n}\sqrt(2\log(2p/(\gamma/\log(n)))$}
     \\
    \emph{(alternative)}&&\\
     \multirow{2}{*}{$X$-dependent}
     & \multirow{2}{*}{$2c\Lambda_W(1-\gamma)$}
     & \multirow{2}{*}{$c\Lambda_W(1-\gamma)$}
     \\
     &&\\
     \hline\hline
    \end{tabular}
    \caption{Lambdas (to add: $\lambda^{lasso}=\lambda_0\hat\sigma$, $\lambda^{sqrt-lasso}=\lambda_0$}
\end{table}    

\begin{table}[H]
    \begin{tabularx}{\linewidth}{lX}
    \hline\hline
    & Estimation of $X$-dependent $\Lambda_W(1-\gamma)$ by simulation
    \\
    \hline
     Homosk.
     & $(1-\gamma)$ quantile of $W$ where $W:=\max_{1 \leq j \leq p} \sum_i (x_{ij} e_i)$, $e_i$ is i.i.d. $N(0,1)$ and independent of $X$, and $x_i$ has been standardized.
     \\
     Heterosk.
     & $(1-\gamma)$ quantile of $W$ where $W:=\max_{1 \leq j \leq p} \sum_i (x_{ij} e_i \frac{\hat\epsilon_i}{\hat\sigma})$, $e_i$ is i.i.d. $N(0,1)$ and independent of $X$, $x_{ij}$ has been standardized, $\hat\epsilon_i$ is a residual and $\hat\sigma$ is an estimate of the variance of the disturbance. 
     \\
     Cluster
     & $(1-\gamma)$ quantile of $W$ where $W:=\max_{1 \leq j \leq p} \sum_i (x_{ijt} e_{i} \frac{\hat\epsilon_{it}}{\hat\sigma})$, $e_i$ is i.i.d. $N(0,1)$, time-invariant (common within clusters) and independent of $X$, $x_{ij}$ has been standardized, $\hat\epsilon_it$ is a residual and $\hat\sigma$ is an estimate of the variance of the disturbance.
     \\
     \hline\hline
    \end{tabularx}
    \caption{Estimation of $X$-dependent $\Lambda_W(1-\gamma)$ by simulation}
\end{table}

\begin{table}[H]
    \begin{tabularx}{\linewidth}{lX}
    \hline\hline
    & Standardized and unstandardized penalty loadings
    \\
    \hline
     Homosk.
     & $\Upsilon^S_j = 1$, $\Upsilon_j = S_j \Upsilon^S_j$, $S_j := \sqrt{ \frac{1}{n}\sum_i (x_{ij}-\Bar{x_j})^2}$
     \\
     Heterosk.
     &  $\Upsilon^S_j = \frac{1}{\hat{\sigma}S_j} \sqrt{\dfrac{1}{n}\sum_i x_{ij}^2 \hat\varepsilon_i^2}$, $\Upsilon_j = S_j \Upsilon^S_j $
     \\
     Cluster
     & 
     \\
     \hline\hline
    \end{tabularx}
    \caption{Estimation of penalty loadings}
\end{table}
